# Supplementary material for: Compositional Inversion for Stable Diffusion Models
Source: arXiv:2312.08048 source file (2024-01-11)
Supplement: Supplementary file 1 [file 1c_supplement.pdf]

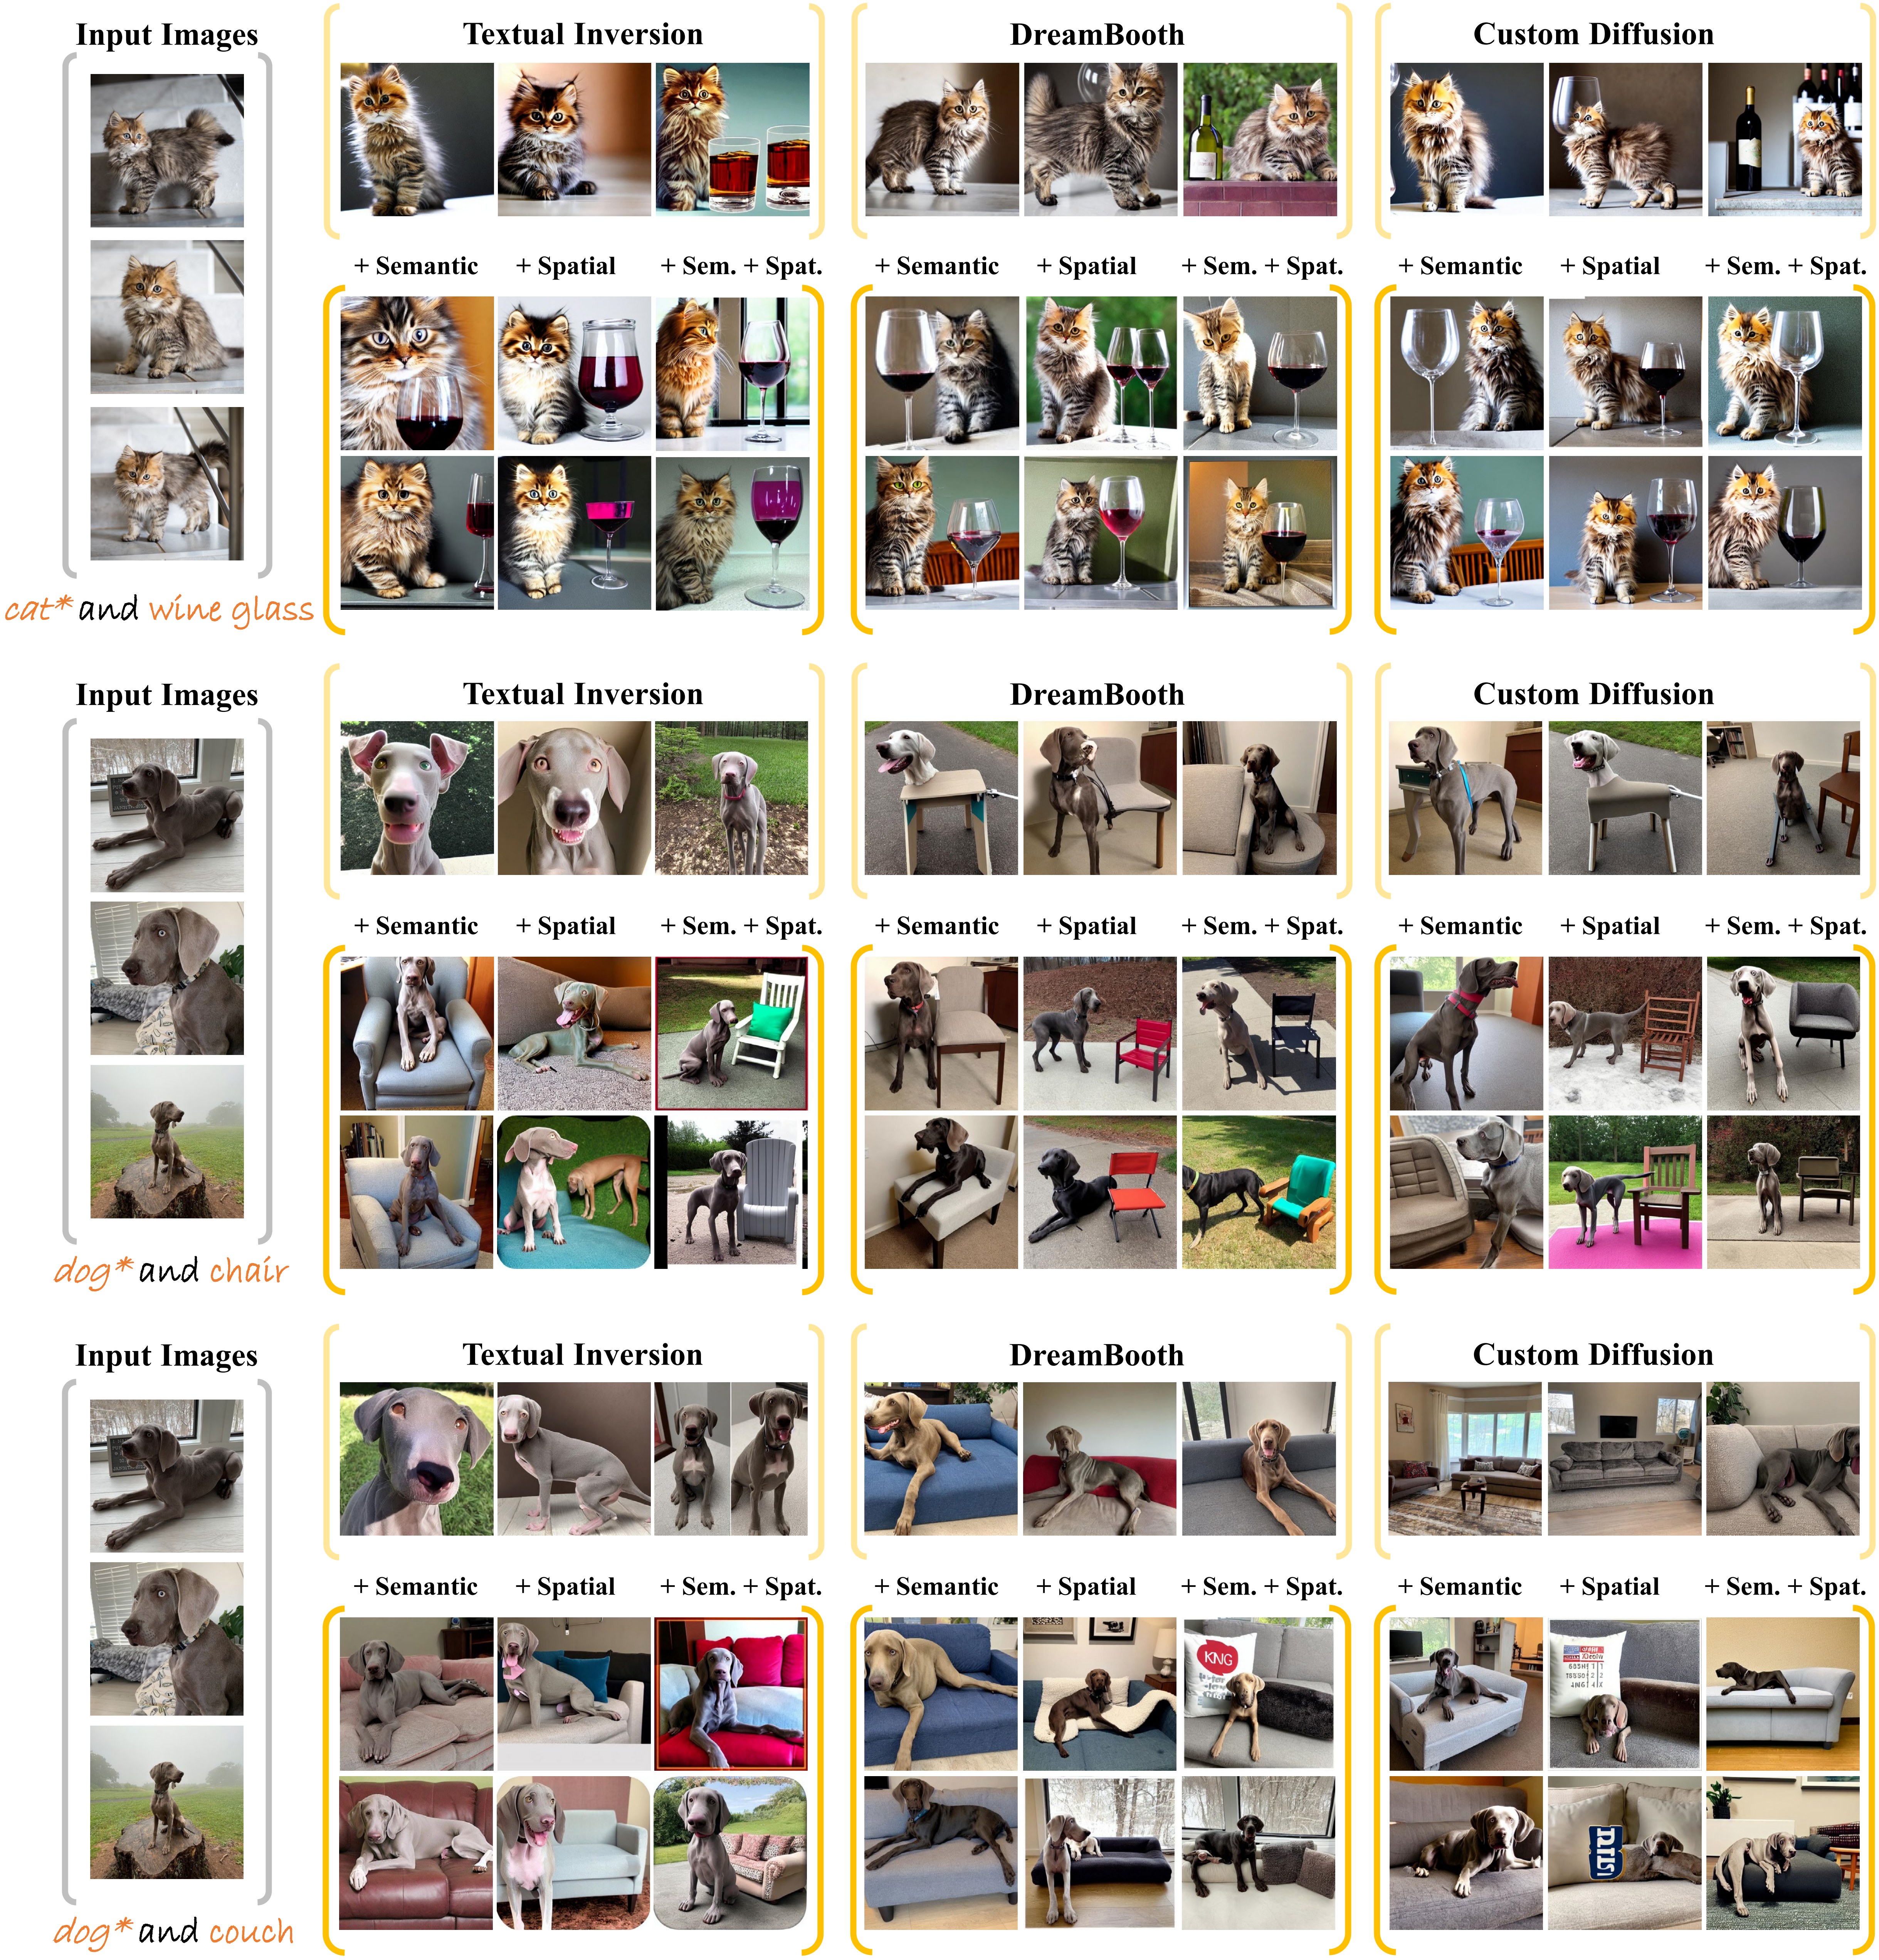
Input Images
Textual Inversion
DreamBooth
Custom Diffusion
+ Semantic
+ Spatial
+ Sem. + Spat.
cat* and wine glass
dog* and chair
dog* and couch

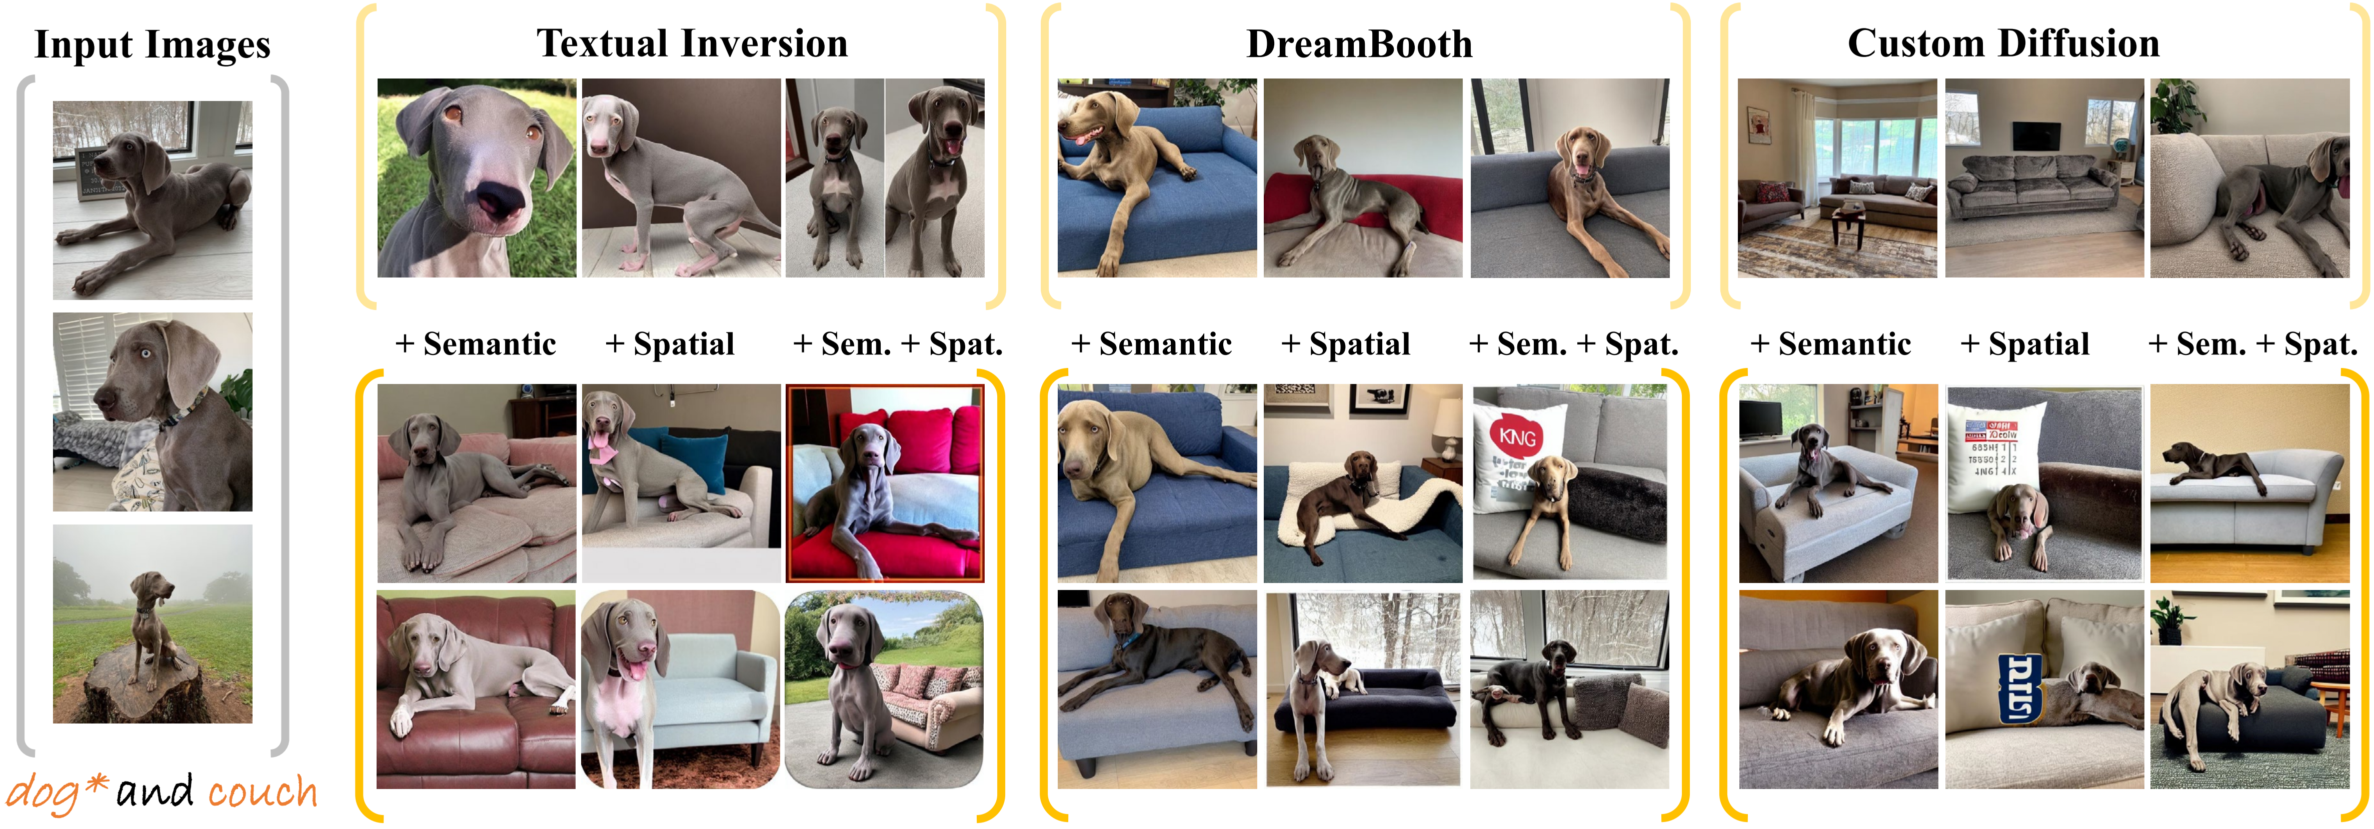
Input Images
Textual Inversion
DreamBooth
Custom Diffusion
+ Semantic
+ Spatial
+ Sem. + Spat.
+ Semantic
+ Spatial
+ Sem. + Spat.
+ Semantic
+ Spatial
+ Sem. + Spat.
dog* and couch

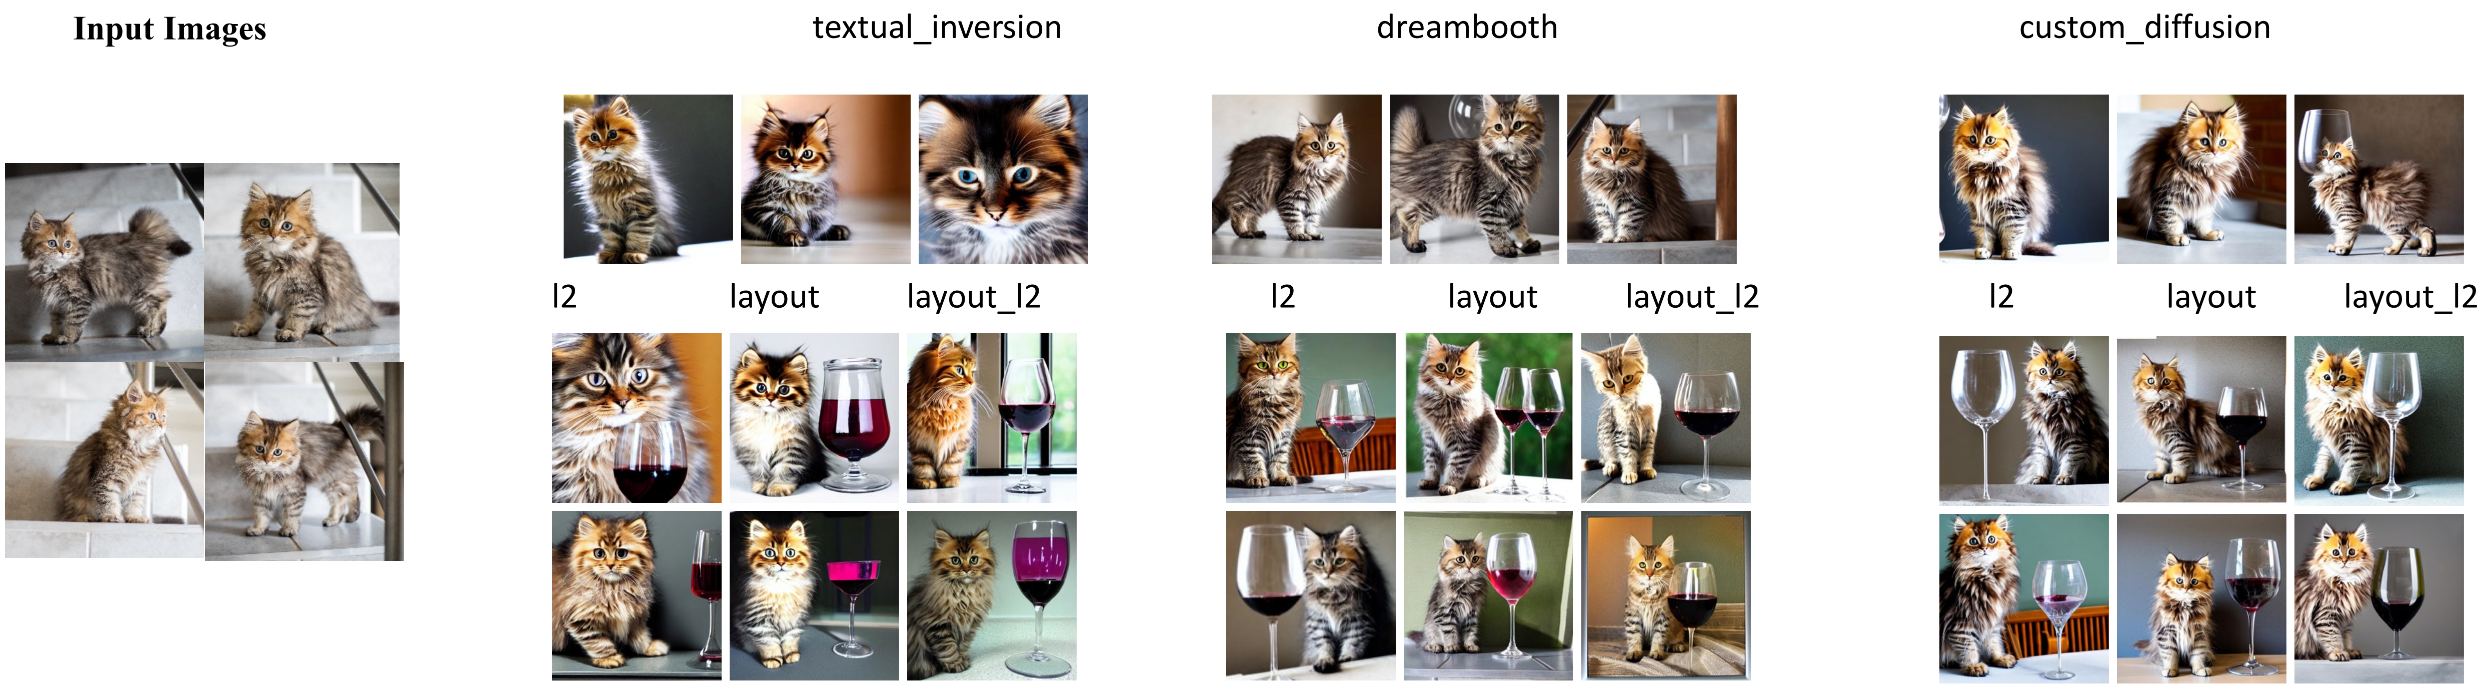


cat and wine glass

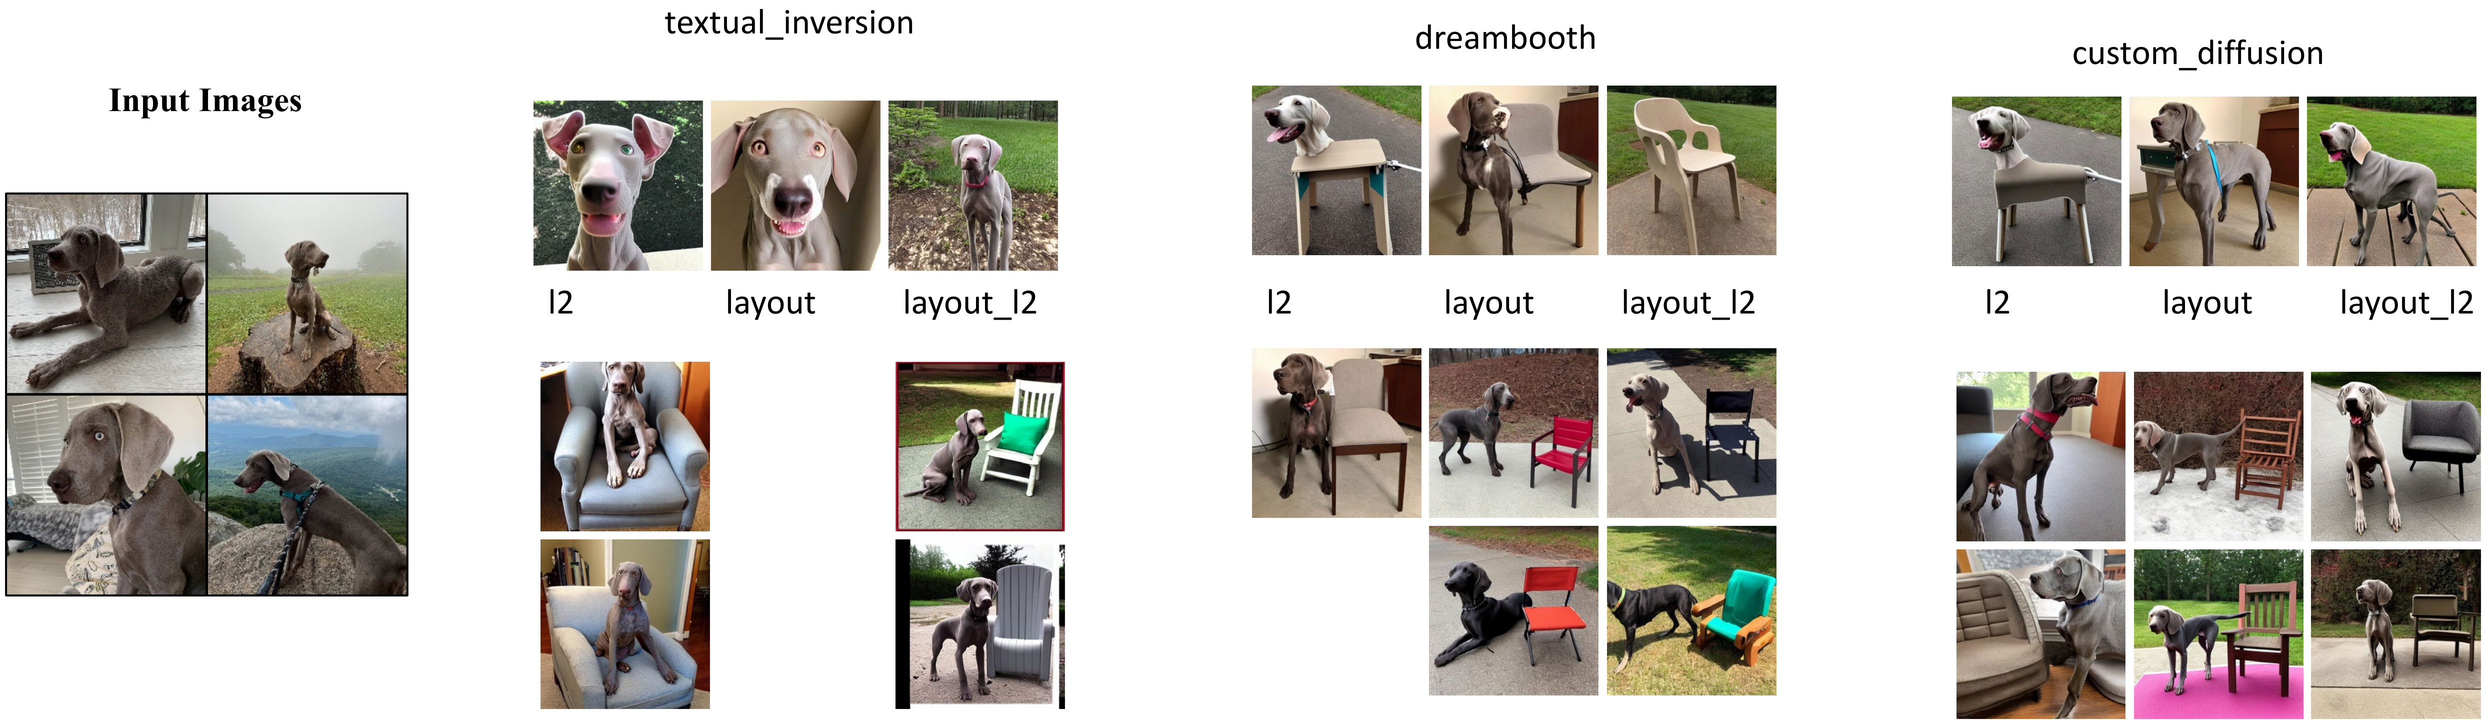


dog and chair

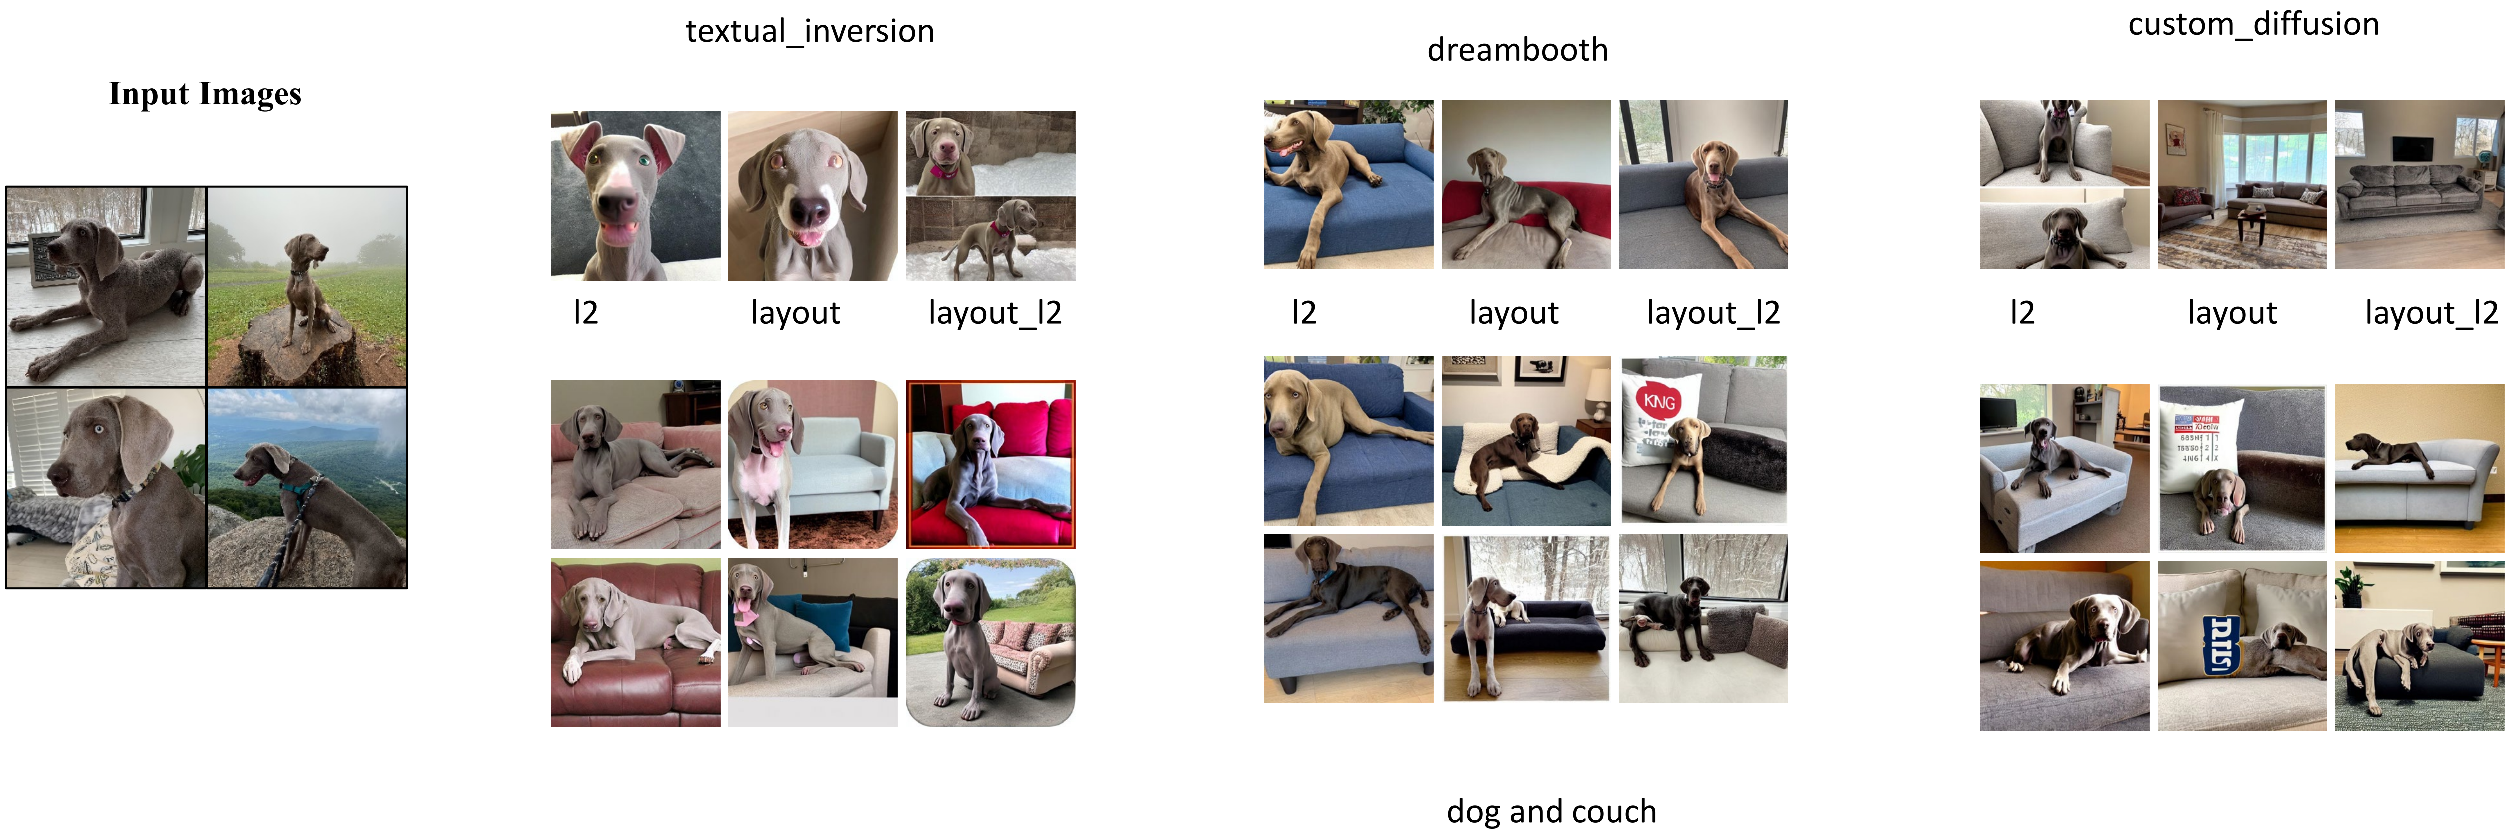
Input Images
textual_inversion
l2
layout
layout_l2
dreambooth
l2
layout
layout_l2
custom_diffusion
l2
layout
layout_l2
dog and couch
