# Supplementary material for: Compositional Inversion for Stable Diffusion Models
Source: arXiv:2312.08048 source file (2024-01-11)
Supplement: Supplementary file 2 [file 2c_supplement.pdf]

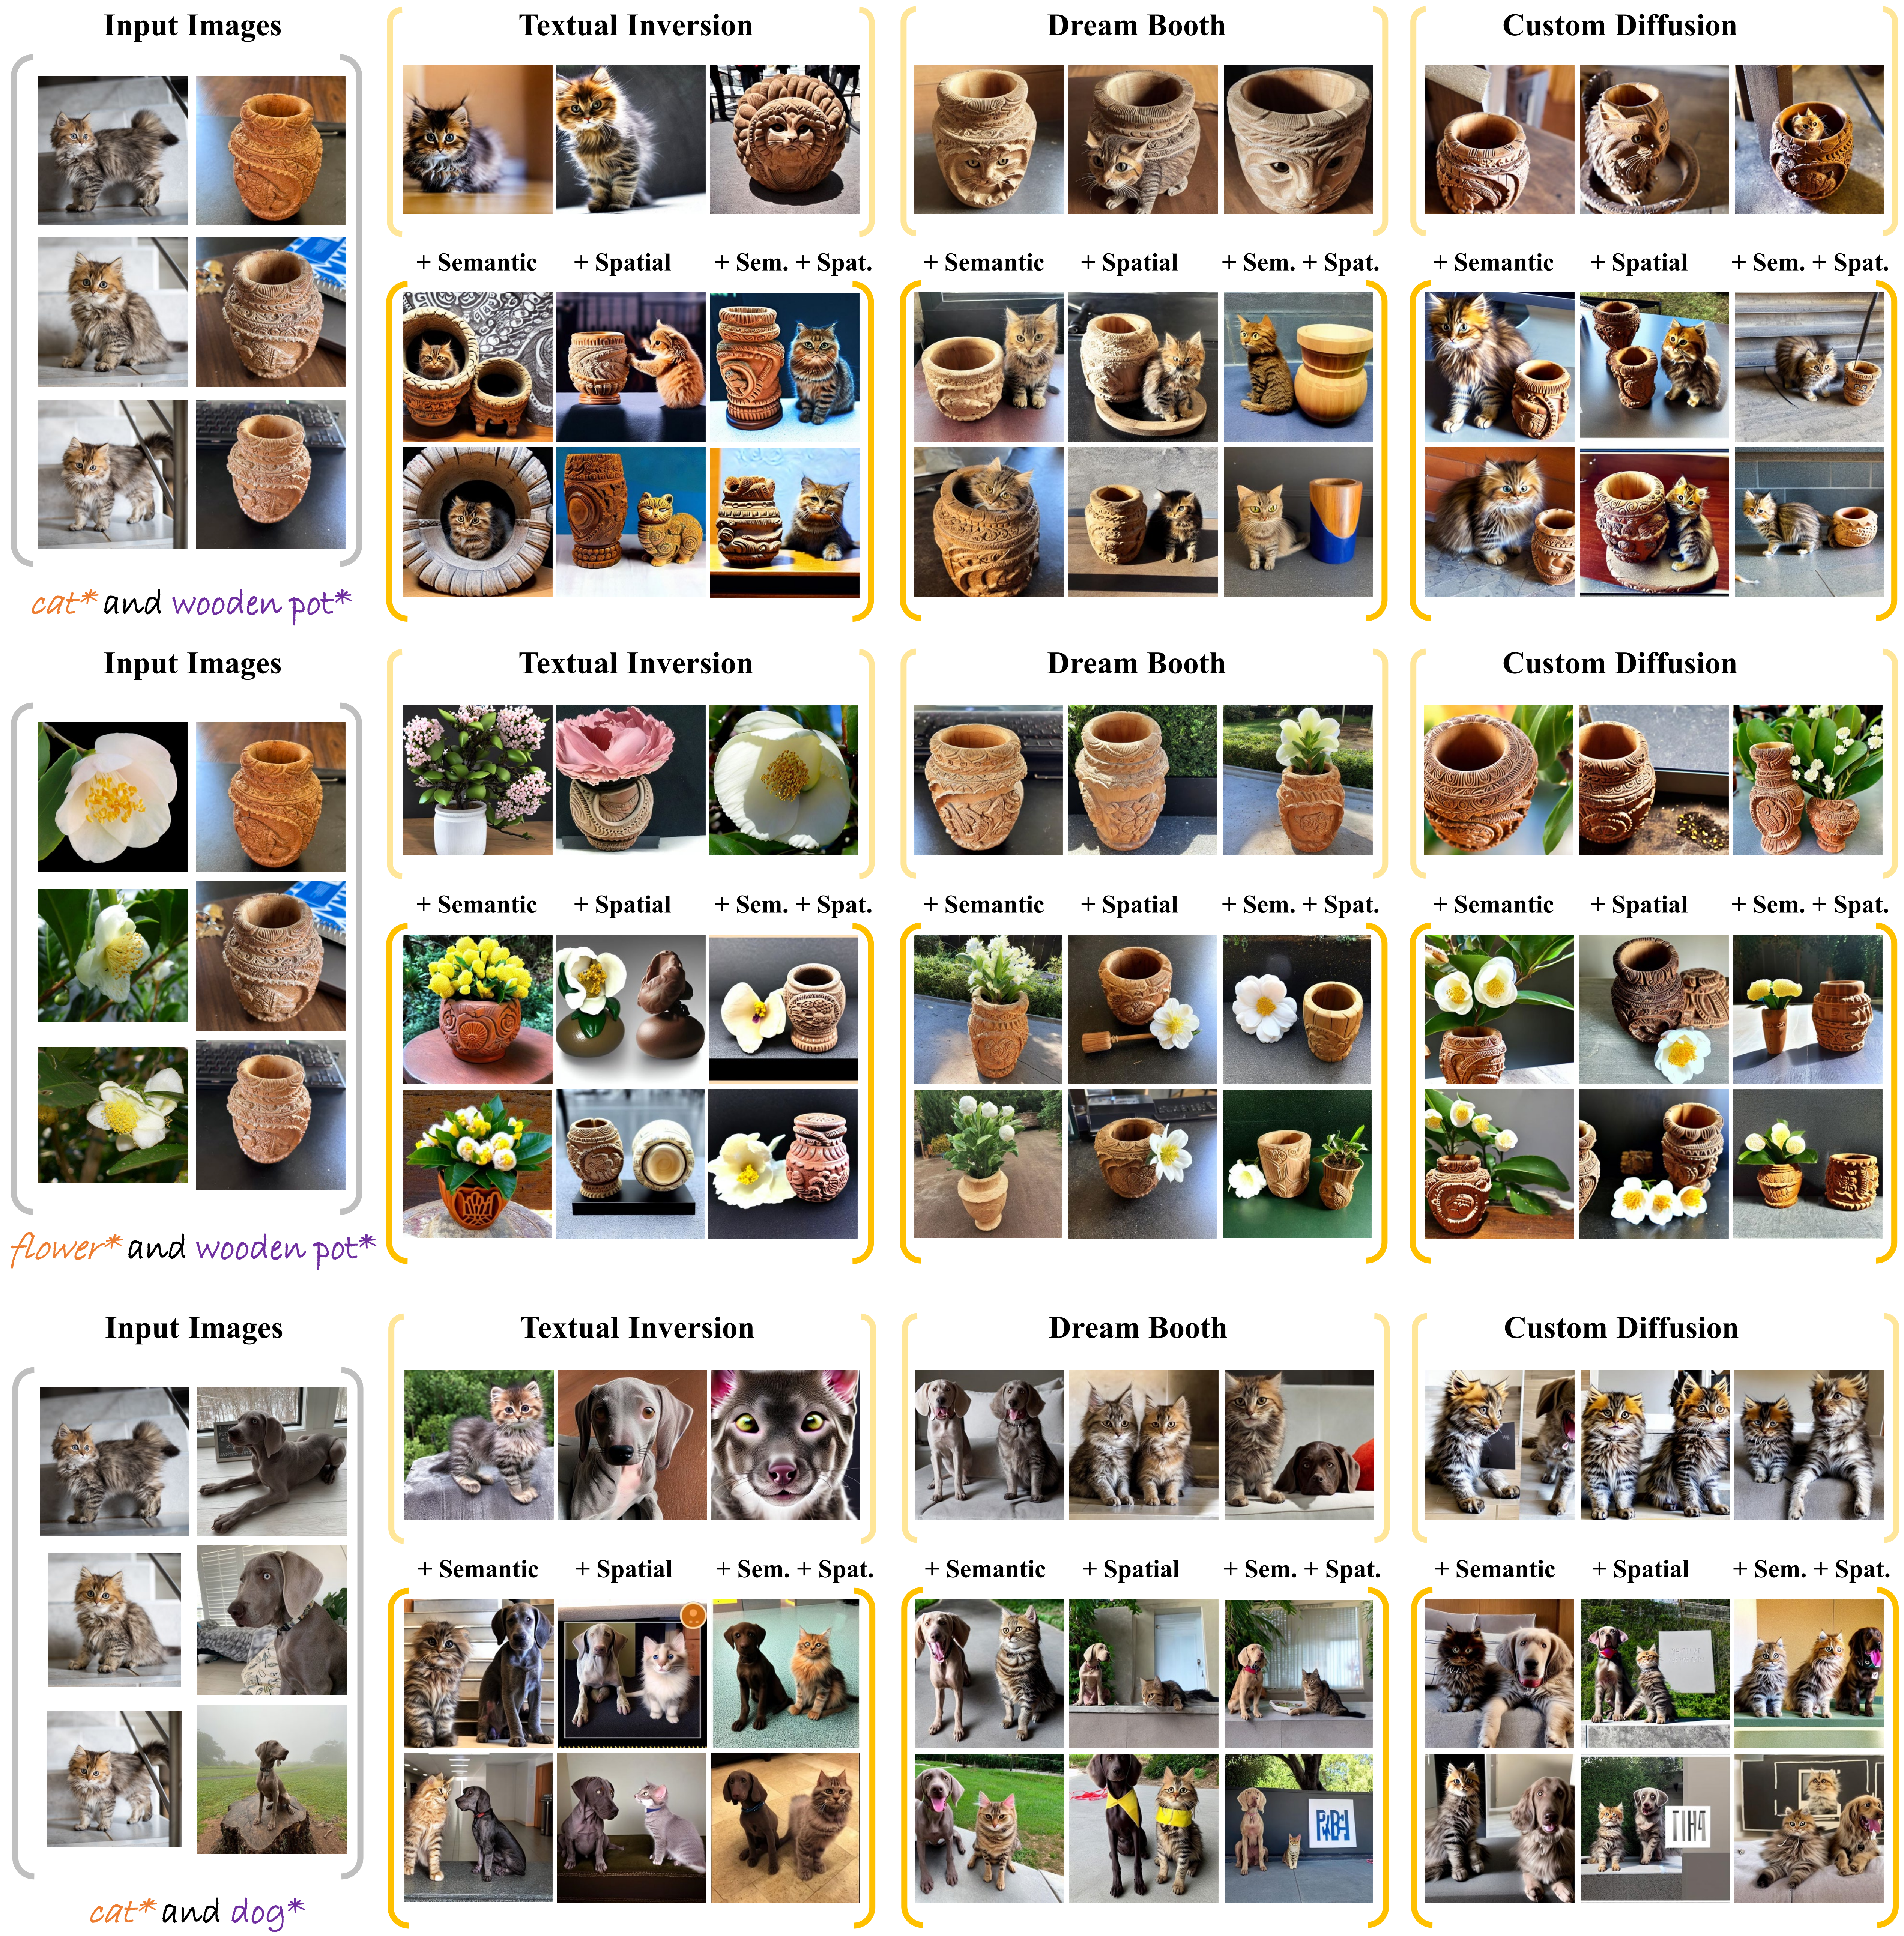
Input Images
Textual Inversion
Dream Booth
Custom Diffusion
+ Semantic
+ Spatial
+ Sem. + Spat.
cat* and wooden pot*
Input Images
Textual Inversion
Dream Booth
Custom Diffusion
+ Semantic
+ Spatial
+ Sem. + Spat.
flower* and wooden pot*
Input Images
Textual Inversion
Dream Booth
Custom Diffusion
+ Semantic
+ Spatial
+ Sem. + Spat.
cat* and dog*

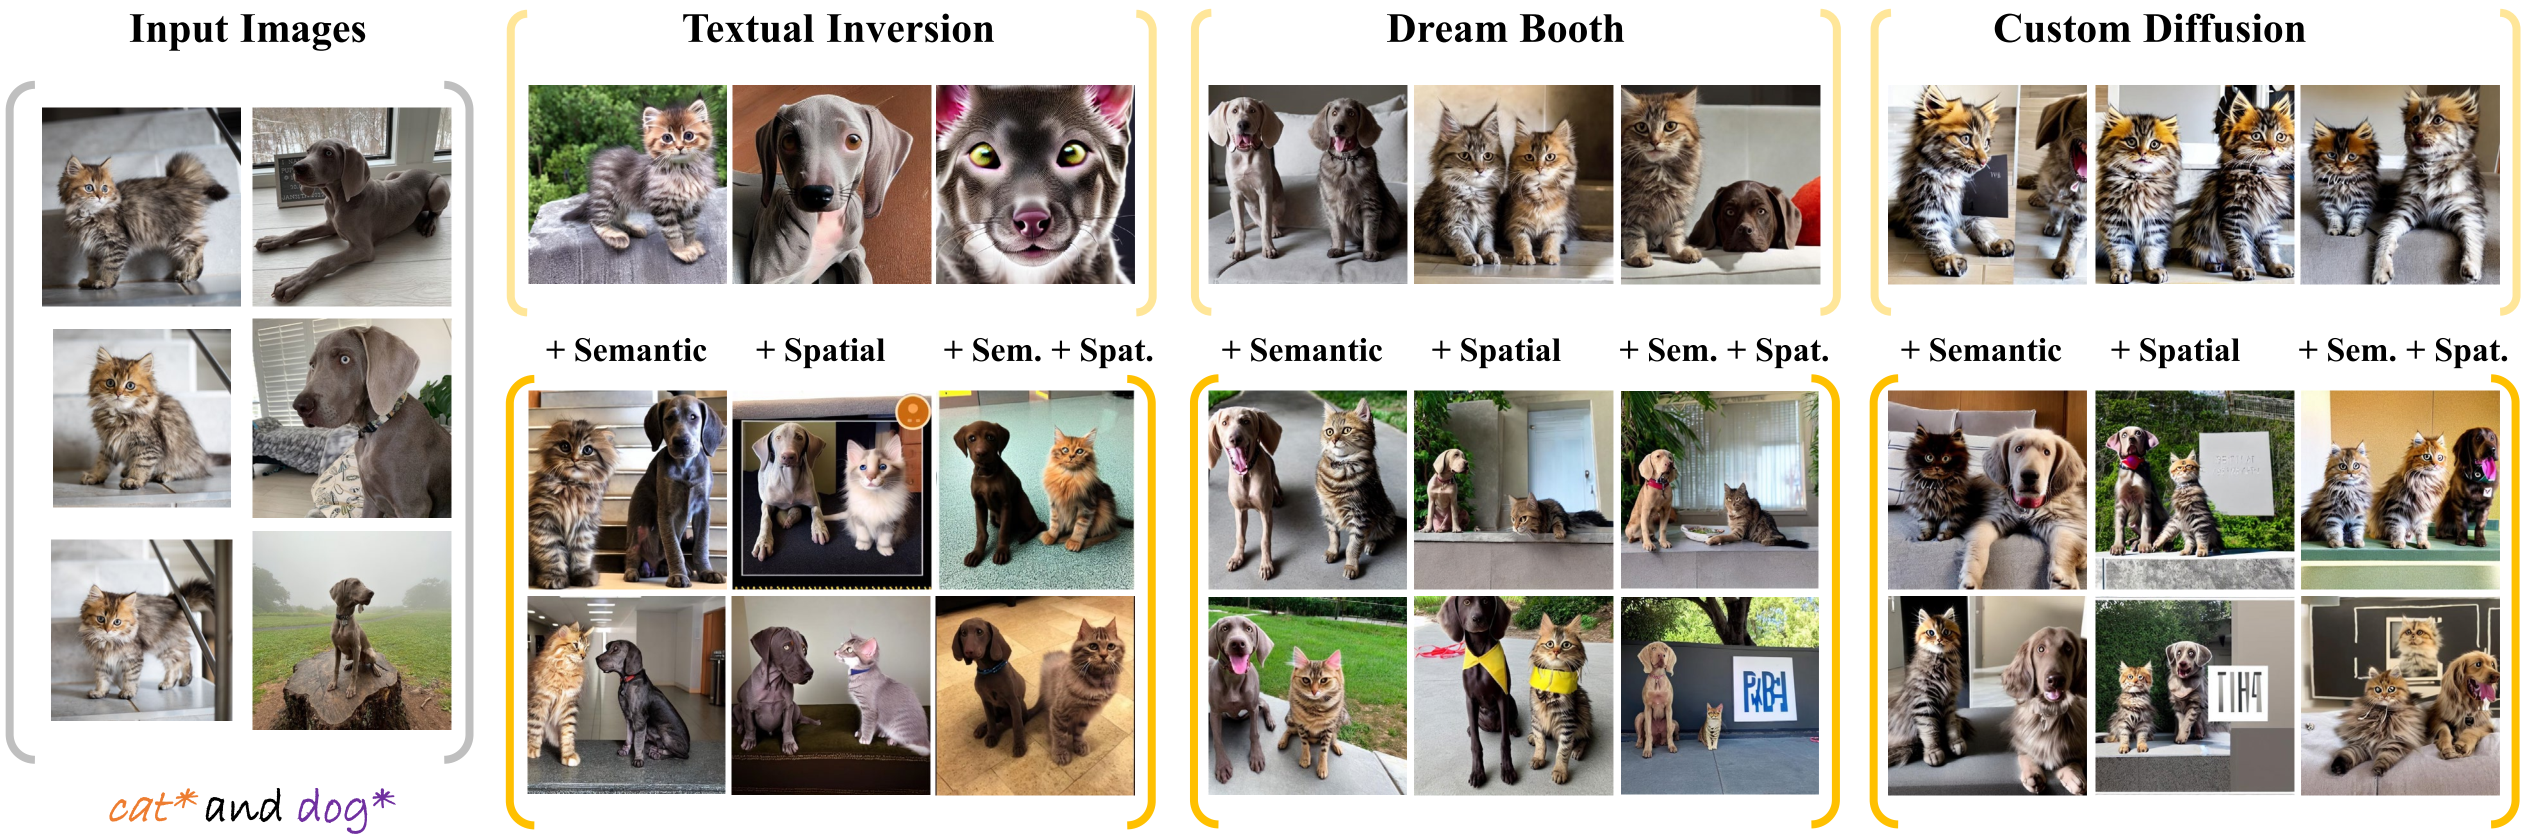
Input Images
Textual Inversion
Dream Booth
Custom Diffusion
+ Semantic
+ Spatial
+ Sem. + Spat.
+ Semantic
+ Spatial
+ Sem. + Spat.
+ Semantic
+ Spatial
+ Sem. + Spat.
cat* and dog*
